# Supplementary material for: Breaking and (Partially) Fixing Provably Secure Onion Routing
Source: arXiv:1910.13772 source file (2019-10-30)
Supplement: Supplementary file 1 [file notionDef.tex]

The model uses $(u,u',m,aux)$ to denote the communication of message $m$ from sender $u$ to receiver $u'$ with auxiliary information $aux$ and it groups communications that are processed together in batches $r_j$.

%The parts that are protected (or not, depending on the notion) are called (communication) properties. Although both are called properties, the communication properties as part of the framework describe characteristics of communications and the security properties as part of the \ac{OR} formalization, we introduced before, describe requirements for private $\ac{OR}$. Here, we introduce the communication properties of~\cite{ownFramework}.

\begin{definition}[Notions\cite{ownFramework}\footnote{We do introduce a shortened definition and do not introduce $\something$ as it is implied by the other requirements.}]
Let the checked batches be $\underline{r_0},\underline{r_1}$,  which  for $b \in \{0,1\}$ include the communications \mbox{${r_b}_j = (u_{b_j},u'_{b_j},m_{b_j},aux_{b_j})$} with $ j \in \{1, \dots l\} $. We say the batches are valid for the privacy notion, iff for all $j \in \{1, \dots l\}$:
\footnotesize
 \begin{align*}
 \conf : & {r_1}_j =(u_{0_j},u'_{0_j},\mathbf{m_{1_j}},aux_{0_j}) \\[0.4em]
 \SML : &{r_1}_j =(\mathbf{u_{1_j}},u'_{0_j},m_{0_j},aux_{0_j}) \land Q\text{, where}\\
Q:& Q_0=Q_1 \text{ for}\\
Q_b:& \{ (u,n) \bigm|  (u,M) \in L_{1}\land |M|=n\}  \text{ with}\\
L_b:=&\{(u,\{m_1,...,m_h\}) \bigm| u \text { sent messages }m_1, \dots , m_h  \text{ in } \underline{r_b}\}\\[0.4em]
 \PairSRL : &{r_1}_j =(\mathbf{u_{1_j}},\mathbf{u'_{1_j}},m_{0_j},aux_{0_j}) \land M_{SR} \text{, where}\\
  M_{SR}& \text{ is defined as in Definition \ref{def:complexProperties}.} \\
 \end{align*}
\end{definition}
To assure that the linking between senders and receivers cannot be learned (Relationship anonymity), the following property lets the adversary pick two senders $A,B$ and two receivers $C, D$. In the case $b=0$ the $A$ and $C$, and $B$ and $D$ communicate with eachother. In the case $b=1$ the $A$ and $D$, and $B$ and $C$ communicate. However, as the order might be noticed by the adversary and she should not be able to win by only learning which receiver belongs to the first communication, the challenger decides the order randomly by picking another bit $a$. Each possible input for the simulation of case $b=0$ is called instance of scenario 0 and thus $a$ is the instance bit. Further, as this definition only cares for communications that differ between the scenarios, they introduce athe term challenge row for communications that differ in both scenarios.

\begin{definition}[Property $M_{SR}$]\label{def:complexProperties}
Let the given batches be $\underline{r}_b^a$ for instances $a \in \{0,1\}$ and scenarios $b \in \{0,1\}$, 
  $\mathsf{CR}$  the set of challenge row indexes, 
  $(u^a_0, {u'}^{\:a}_0)$ for both instances $a\in \{0,1\}$  be the sender-receiver-pairs of the first challenge row of the first scenario ($b=0$).
Mixed Sender Receiver $M_{SR}$ ($M_{SM}, M_{RM}$ analogous) are met, iff:
\allowdisplaybreaks
\begin{align*}
      M_{SR}:\quad&{r_0^a}_{cr}=(\mathbf{u^{a}_0}, \mathbf{ {u'}^{\:a}_0},m^1_{0_{cr}},aux^1_{0_{cr}})~\land \\
   &{r_0^a}_{cr+1}= (\mathbf{u^{1-a}_0}, \mathbf{ {u'}^{\:1-a}_0}, m^1_{0_{cr}},aux^1_{0_{cr}})~\land \\[0.2em]
   &{r_1^a}_{cr}=(\mathbf{u^{a}_0}, \mathbf{ {u'}^{\:1-a}_0},m^1_{0_{cr}},aux^1_{0_{cr}})~\land \\
   &{r_1^a}_{cr+1}=(\mathbf{u^{1-a}_0},\mathbf{ {u'}^{\:a}_0}, m^1_{0_{cr}},aux^1_{0_{cr}})\\[0.2em]
   &\text{for every second } cr \in \mathsf{CR} , a \in \{0,1\}& 
\end{align*}
%\todo[inline]{The last cr has to skip every second cr.. How to write this?}

\end{definition}

$X_{c^0}$ ensures that the adversary is not allowed to send any corrupt(user) -query. Other user corruption with $\hat{U}$ as the set of all users corrupted via such queries is defined as follows:
\begin{definition}[Corruption]\label{def:corruption}
The following properties are met, iff for all $a \in \{0,1\}$:
{\footnotesize
\begin{align*}
  %\corrNoComm{corr}&: \forall (u,u',m,aux) \in \underline{r}^a_0\cup \underline{r}^a_1: u \not \in \hat{U} \land u' \not \in \hat{U} \\
  \corrOnlyPartnerSender{corr}&: \forall (u,u',m,aux) \in \underline{r}^a_0\cup \underline{r}^a_1: u \not \in \hat{U} \\
  \corrOnlyPartnerReceiver{corr}&: \forall (u,u',m,aux) \in \underline{r}^a_0\cup \underline{r}^a_1: u' \not \in \hat{U}\\
  \corrStandard{corr}&: \forall \hat{u} \in \hat{U}:r^a_{0_i}=(\hat{u},\_,m,\_) \implies r^a_{1_i}=(\hat{u},\_,m,\_)\\
   &\quad \quad \quad \quad \land r^a_{0_i}=(\_,\hat{u},m,\_) \implies r^a_{1_i}=(\_,\hat{u},m,\_) \\
\end{align*}
}
\end{definition}
