# Supplementary material for: Breaking and (Partially) Fixing Provably Secure Onion Routing
Source: arXiv:1910.13772 source file (2019-10-30)
Supplement: Supplementary file 3 [file originalDef.tex]

\subsubsection{Onion-Correctness~\cite{camenisch2005formal}}

\begin{definition}{Onion-correctness} Let \((G, FormOnion, ProcOnion)\) satisfy
the I/O spec for an onion routing scheme. Then for all settings of the public
parameters $p$, for all $n < N$ , and for all $Q$ with a public-key infrastructure
as in Definition 2, for any path $P = (P_1 , . . . , P_{n+1} )$,$P \subseteq Q$, for all messages
$m \in M (1\lambda)$, and for all onions $O_1$ formed as
\((O_1, . . . , O_{n+1} )\gets FormOnion(m, N, (P_1 , . . . , P_{n+1} ), (PK(P_1 ), . . . , PK(P_{n+1} )))\)
the following is true: (1) correct path: \(P(O_1, P_1) = (P_1, . . . , P_{n+1} )\); (2) cor-
rect layering: \(L(O_1 , P_1 ) = (O_1 , . . . , O_{n+1})\); (3) correct decryption: \((m, \perp) =
ProcOnion(SK(P_{n+1} ), O_{n+1}, P_{n+1} )\).
\end{definition}

\subsubsection{Wrap-Resistance~\cite{camenisch2005formal}}
\begin{definition}[wrap-resistance]\label{def:wrapResistance}
  Consider an adversary interacting with an onion routing challenger as follows.
  
  \begin{enumerate}
    \item The adversary receives as input a challenge public key \(PK\), chosen by the challenger by letting \((PK,SK) \leftarrow G(1^{\lambda}, p)\), and the router name \(P\).
    \item The adversary submits any number of onions \(O_i\) of his choice to the challenger, and obtains the output of \(\mathrm{ProcOnion}(SK, O_i, P)\).
    \item The adversary submits \(n\), a message \(m\), a set of router names \((P_1,\ldots,P_{n+1})\), an index \(j\), and \(n\) key pairs \(1 \leq i \leq n, i \neq j, (PK_i, SK_i)\).
      The challenger checks that the router names are valid, that the public keys correspond to the secret keys and if so, sets \(PK_j = PK\), sets bit \(b\) at random and does the following:
      \begin{itemize}
        \item If \(b=0\), let
          \((O_1,\ldots,O_j,\ldots,O_{n+1}) \leftarrow \mathrm{FormOnion}(m,(P_1,\ldots,P_{n+1}),(PK_1,\ldots,PK_{n+1}))\)
        \item Otherwise, choose \(r \leftarrow M(1^{\lambda})\), and let
          \((O_1,\ldots,O_j) \leftarrow \mathrm{FormOnion}(r,(P_1,\ldots,P_{j}),(PK_1,\ldots,PK_{j}))\)
      \end{itemize}
      The challenger returns \(O_1\) to the adversary.
    \item The adversary may submit any number of onions \(O_i \neq O_j\) of his choice to the challenger, and obtain the output of \(\mathrm{ProcOnion}(SK, O_i, P)\).
    \item The adversary submits a secret key \(SK'\), an identity \(P' \neq P_{j-1}\), and an onion \(O'\).
      If \(P'\) is valid and \(SK',O',P'\) satisfy the condition \(O_j=\mathrm{ProcOnion}(SK',O',P')\) he wins the game.
  \end{enumerate}
    
  We say that a scheme with onion routing I/O satisfies onion wrap-resistance if for all probabilistic time adversaries \(A\) of the form described above, there is a negligible function \(v\) such that the adversary's probability of submitting a secret key \(SK'\), an onion \(O'\) and an identity \(P'\) which fulfill above conditions is at most \(v(\lambda)\).
\end{definition}

\subsubsection{Onion-Integrity~\cite{camenisch2005formal}}
\begin{definition}[Onion-integrity]\label{def:onionIntegrity}
  (Sketch) An onion routing scheme satisfies onion-integrity if for all probabilistic polynomial-time adversaries, the probability (taken over the choice of the public parameters \(p\), the set of honest router names \(\mathcal{Q}\) and the corresponding PKI as in Definition \(2)\)~\cite{camenisch2005formal} that an adversary with adaptive access to \(\mathrm{ProcOnion}(SK(P ), \cdot, P )\) procedures for all \(P \in \mathcal{Q}\), can produce and send to a router \(P_1 \in \mathcal{Q}\) an onion \(O_1\) such that \(|\mathcal{P}(O_1,P_1)| > N\) , is negligible.
\end{definition}

\subsubsection{Onion-Security~\cite{camenisch2005formal}}
\begin{definition}[Onion-Security]\label{def:onionSecurity}
  Consider an adversary interacting with an onion routing challenger as follows.
  \begin{enumerate}
    \item - 4) as in Definition~\ref{def:wrapResistance}
    \addtocounter{enumi}{3}
    \item The adversary then produces a guess $b'$.
  \end{enumerate}
        
  We say that a scheme with onion routing I/O satisfies onion security if for all probabilistic time adversaries \(A\) of the form described above, there is a negligible function \(v\) such that the adversary's probability of outputting $b'=b$ is at most \(\frac{1}{2}+v(\lambda)\).
\end{definition}
